# Supplementary material for: Striking a Balance: Evaluating How Aggregations of Multiple Forecasts Impact Judgment Under Uncertainty
Source: arXiv:2411.02576 source file (2026-01-27)
Supplement: Supplementary file 1 [file 8-appendix.tex]

% \newpage
% \section*{Appendix: }
% \label{appendix:}

\input{tabs/results-full}
